# Supplementary material for: Modelling of shattered pellet injection experiments on the ASDEX Upgrade tokamak
Source: arXiv:2312.03462 source file (2023-12-06)
Supplement: Supplementary file 1 [file Appendix.tex]

\newpage
\section{Appendix}

\subsection*{Additional plots}

\subsection*{Discharge numbers for experimental pre-TQ duration}
Discharge numbers of data points in \autoref{fig:v_normal_vs_Pre_TQ_all_neon_subplots} and \autoref{fig:v_para_vs_Pre_TQ_all_neon_subplots} grouped by the shattering tube used:
\begin{itemize}
    \item \textbf{10\% Neon}
    GT1 ($25^\circ$ (rect.)): 40673
    GT2 ($25^\circ$ (circ.)): 40674, 40951
    GT3 ($12.5^\circ$ (rect.)): 40671, 40785, 40786, 40949, 40952, 40990, 40997
    \item \textbf{40\% Neon}
    GT1 ($25^\circ$ (rect.)): 40675
    GT2 ($25^\circ$ (circ.)): 40676
    GT3 ($12.5^\circ$ (rect.)): 40677, 40783, 40784
\end{itemize}
